# Supplementary material for: Isotropic and Anisotropic g-factor Corrections in GaAs Quantum Dots
Source: arXiv:2010.11185 ancillary file (2020-10-21)
Supplement: Supplementary file 1 [file SOM.pdf]

# Supplemental Material
# Isotropic and Anisotropic g-factor Corrections in GaAs Quantum Dots

Leon C. Camenzind,[1,*] Simon Svab,[1,*] Peter Stano,[2,3] Liuqi Yu,[1,†] Jeramy D. Zimmerman,[4,‡] Arthur C. Gossard,[4] Daniel Loss,[1,2] and Dominik M. Zumbühl[1]

[1]*Department of Physics, University of Basel, Basel 4056, Switzerland*
[2]*Center for Emergent Matter Science, RIKEN, Saitama 351-0198, Japan*
[3]*Institute of Physics, Slovak Academy of Sciences, 845 11 Bratislava, Slovakia*
[4]*Materials Department, University of California, Santa Barbara 93106, USA*
(Dated: 10 / 12 / 2020)

## CONTENTS

Supplemental Section 1: Comparison of wafer properties in the two devices 2

Supplemental Section 2: Influence of the dot shape on the $g$-factor corrections 3

Supplemental Section 3: Tunnel rate into the spin states 4

Supplemental Section 4: Suppression of the tunnel rate in a magnetic field 5

Supplemental Section 5: $g$-factor corrections in device 2 6

References 7

## SUPPLEMENTAL SECTION 1: COMPARISON OF WAFER PROPERTIES IN THE TWO DEVICES

A schematic of the wafer profiles in our samples is shown in Fig. S1. The wafer of device 2 has a decreased mobility and density of remote Si dopants compared to that of device 1. The following values for the mobility $\mu$, the 2DEG density $n$ and the dopant density $n_\delta$ were measured in the two wafers:

| | $\mu\ [\frac{cm^2}{V\cdot s}]$ | $n\ [cm^{-2}]$ | $n_\delta\ [cm^{-2}]$ |
|---|---|---|---|
| Device 1 (Gossard-060926C) | $4 \cdot 10^5$ | $2.6 \cdot 10^{11}$ | $6 \cdot 10^{12}$ |
| Device 2 (Gossard-060926B) | $2.8 \cdot 10^5$ | $2.8 \cdot 10^{11}$ | $4 \cdot 10^{12}$ |

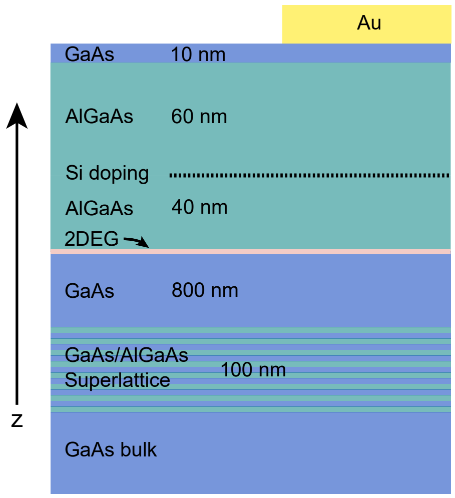


FIG. S1. Schematic representation of the GaAs/AlGaAs heterostructures used in the experiment. 110 nm below the surface, a two-dimensional electron gas (2DEG) is formed at the GaAs/AlGaAs interface. Silicon atoms in a $\delta$-doping layer serve as a remote doping, providing electrons to the 2DEG.

## SUPPLEMENTAL SECTION 2: INFLUENCE OF THE DOT SHAPE ON THE $g$-FACTOR CORRECTIONS

By using the spectroscopy of quantum dot orbitals with in-plane magnetic fields (see Ref. [1]), the following values for the orbital excitation energies $E_{x,y,z}$ and corresponding confinement lengths $l_{x,y,z}$ were extracted in the two devices:

| | $E_x$ [meV] | $E_y$ [meV] | $E_z$ [meV] | $l_x$ [nm] | $l_y$ [nm] | $l_z$ [nm] |
|---|---|---|---|---|---|---|
| Device 1 | 1.9 | 2.6 | 28.6 | 24.5 | 20.9 | 6.3 |
| Device 2 | 1.7 | 3 | 25.5 | 25.8 | 19.5 | 6.7 |

We find that the quantum dot in device 2 is closer to the condition $E_y \approx 2E_x$ than in device 1, indicating an elongated quantum dot close to the quasi-one-dimensional limit. While this difference in the dot shape changes the predicted behaviour of the quantum dot orbitals [2], its effect on the g-factor corrections in the theoretical framework of Ref. [3] is negligible. The reason for this behaviour is that the g-factor corrections merely depend on the energy $E_z$, which is given by the interface electric field of the heterostructure, rather than $E_x$ and $E_y$. The weak effect of the dot shape on the g-factor corrections is shown in Fig. S2, where the dependence of the predicted g-factor on the in-plane magnetic field direction is shown for the dot shape in device 1 (red curve) and device 2 (blue curve). The predicted g-factor differences for the two dot shapes are far smaller than what can be resolved in the experiment.

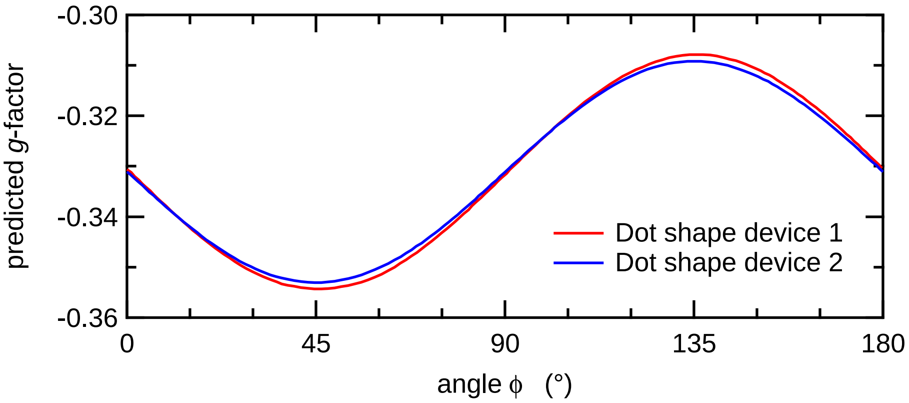


FIG. S2. Theoretical predictions for the g-factor in dependence of the angle $\phi$ of the in-plane magnetic field for the dot shapes found in device 1 (red) and device 2 (blue).

## SUPPLEMENTAL SECTION 3: TUNNEL RATE INTO THE SPIN STATES

Here, we discuss a qualitative model for $\Gamma(\Delta E)$. This phenomenological model is used to explain $\Gamma(\Delta E)$ as discussed and shown in Fig. 2a of the main text. The spin degeneracy of the ground state is lifted in an external magnetic field, such that the ground ($|\uparrow\rangle$) and the excited spin state ($|\downarrow\rangle$) become energetically separated by the Zeeman energy $\Delta$. When occupied states in the reservoir are aligned with empty levels of the quantum dot, an electron can elastically tunnel into the empty quantum dot [4]. In this situation, the tunnel rate $\Gamma$ is defined by a combination of three factors: the density of electrons capable of tunneling into the quantum dot, the number of quantum dot levels into which these electrons could tunnel and the details of the tunnel barrier. At zero temperature and when ignoring any energy dependence of the tunnel barrier, $\Gamma(\Delta E)$ rises to the ground state tunnel rate $\Gamma_g$ when $E_0$ is aligned with $\mu$ at $\Delta E = 0$ (see Fig. 2a of the main text). Upon increasing $\Delta E$ further, $\Gamma(\Delta E) = \Gamma_g$ until tunneling into the spin excited state becomes energetically allowed at $\Delta E = \Delta$ such that $\Gamma(\Delta E) = \Gamma_g + \Gamma_e$ where $\Gamma_e$ is the tunnel rate into the spin excited state.

At a finite temperature, the states in the reservoir are occupied according to the Fermi-Dirac distribution $f(E, k_B T) = 1/\left(\exp\left(\Delta E/(k_B T)\right) + 1\right)$ where $k_B$ is the Boltzmann constant and $T$ is the temperature. This thermal occupation factor, $f(E, k_B T)$, is identified in the data close to zero detuning $\Delta E = 0$ and at the Zeeman splitting $\Delta E = \Delta$, as a broadening of the resonance condition when $\mu$ is aligned with $|\uparrow\rangle$ and $|\downarrow\rangle$, respectively.

Further, the tunnel barrier potential leads to a suppression of $\Gamma$ with increasing $\Delta E$ because the electrons have to tunnel through a larger potential [4–7]. This energy dependence is reflected in the WKB expression for the tunnel rate of a particle with energy $E$ through a potential barrier of height $V_0$. For small energies $\Delta E \ll V_0$, this expression can be simplified to $\Gamma(\Delta E) \sim \Gamma_0 e^{-\beta \Delta E}$ (see Supplemental Section 4) where $\Gamma_0$ and $\beta$ depend on the details of the tunnel barrier potential [4].

In summary, for small detunings $\Delta E$, the tunnel rate can then be expressed as

$$\begin{aligned}\Gamma(\Delta E) &= \Gamma_g(\Delta E) + \Gamma_e(\Delta E) \\ &= \Gamma_0 e^{-\beta \Delta E} \left[ f(\Delta E, k_B T) + \chi f(\Delta E + \Delta, k_B T) \right],\end{aligned} \tag{S1}$$

where $\chi$ is an empirically introduced ratio between $\Gamma_e$ and $\Gamma_g$ [5]. From symmetry arguments one would expect $\Gamma_e = \Gamma_g$: in a magnetic field, the ground state of the quantum dot and the conduction band both split by the Zeeman energy $\Delta$. As a consequence, the tunnel barrier for electrons of both spin species should be equal ($\chi = 1$). While not discussed in this article, in the experiment we often find spin dependent tunnel rates such that $\chi < 1$ [8, 9]. The cause of this asymmetry is not understood conclusively yet [6].

At some configurations of the magnetic field, fitting of our data to Eq. S1 was difficult due to suppressed tunneling into the excited spin state and reservoir resonances. In such cases, the Zeeman splitting could be extracted by fitting sigmoid functions to the thermally broadened spin transitions. Alternatively, for some of the data points in device 2 a better fit could be obtained when using two separate factors $\beta_1$ and $\beta_2$ for the two spin states [4]. These fit procedures result in very comparable Zeeman energies $\Delta$ – the quantity in which we are interested in for this work.

## SUPPLEMENTAL SECTION 4: SUPPRESSION OF THE TUNNEL RATE IN A MAGNETIC FIELD

In Ref. [2] we found a mass renormalization due to an in-plane magnetic field $B_{\parallel}$ of

$$\frac{1}{m^*} \approx \frac{1}{m^*(\Phi = 0)} \left( \frac{1}{1 + \Phi^2} \right). \tag{S2}$$

Here, $\Phi = \frac{e}{\hbar} B_{\parallel} \lambda_z^2$ is the flux due to $B_{\parallel}$ through the 2DEG effective width $\lambda_z$ squared. For simplicity, we only focus on corrections due to the confinement along the growth direction.

For an electron tunneling through a rectangular potential barrier, the transmission coefficient is [10]

$$T(E) \propto \exp\left( \frac{-2 \cdot d}{\hbar} \sqrt{2m^* \left(U_0 - \mu + \Delta E\right)} \right), \tag{S3}$$

where $d$ is the width and $U_0$ the height of the tunnel barrier (see Fig. S3a). For small energies $\Delta E$, one can simplify the exponent $T(E) \propto \exp\left( -\sqrt{2m^* \cdot (U_0 - \mu + \Delta E)} \right) \rightarrow T(E) \propto \exp\left(-\beta \Delta E\right)$ [4]. Using Eq. (S2) in Eq. (S3) gives

$$T(E) \propto \exp\left( \frac{-2d}{\hbar} \sqrt{2 \cdot m^*(B = 0) \left(1 + \frac{e^2}{\hbar^2} \cdot B_{\parallel}^2 \lambda_z^4\right) \left(U_0 - \mu + \Delta E\right)} \right). \tag{S4}$$

In Fig. S3b we show the exponential decay of the tunnel rate $\Gamma_0$ in an in-plane magnetic field $B_{\parallel}$ due to an increase of the effective mass. We obtain excellent agreement with the model given in Eq. (S4) and find $d \sim 66$ nm when using $U_0 - \mu \sim 5$ meV [4]. This data was taken in a device with a different gate layout [11] that was fabricated on the same wafer material as device 1 of our experiment. In contrast to the data presented in the main text, no adjustments of the voltages defining the tunnel barrier were made here. However, to compensate for orbital effects on the quantum dot, the voltage on the plunger gate was slightly adjusted for measurements at different fields. We do not expect any significant change of the shape or position of the quantum dot for these small adjustments. The tunnel rates $\Gamma_0$ were obtained by analyzing real-time traces of resonant tunneling at zero detuning ($\Delta E = 0$) where $f(E, k_B T) = 0.5$.

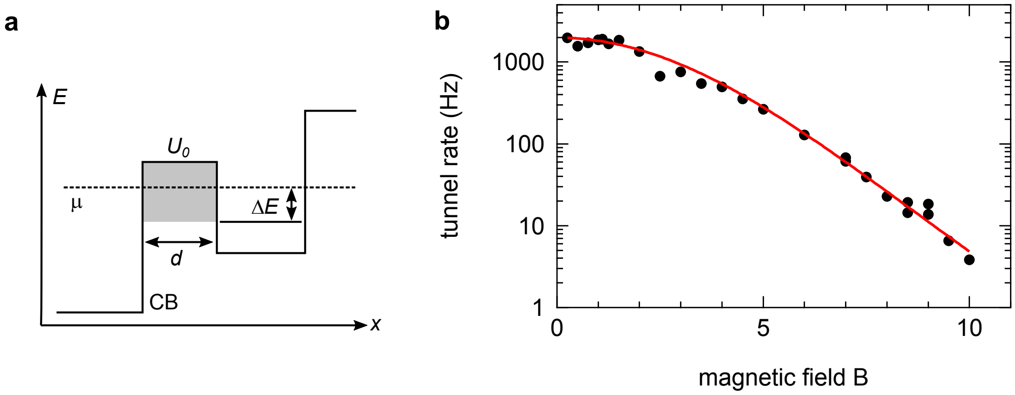


FIG. S3. (a) Simplified schematic of the tunnel barrier defined by a modulation of the conduction band (CB) potential by means of gate voltages. The electrostatically defined quantum dot is represented by its orbital ground state energy detuned by $\Delta E$ from the chemical potential $\mu$. (b) The tunnel rate $\Gamma_0$ decays exponentially with magnetic field strength because of the increase of effective mass. Data taken for $B \parallel Y$ in another device which was fabricated on the same 2DEG material as device 1.

## SUPPLEMENTAL SECTION 5: $g$-FACTOR CORRECTIONS IN DEVICE 2

In this section, we present the measured g-factor corrections for device 2. In Fig. S4, the extracted Zeeman splittings $\Delta E_Z$ for different in-plane magnetic field angles $\phi$ are plotted in dependence of $\mu_B B$, which allows us to extract the absolute g-factor $|g|$ by fitting with a linear function. The measurements for this device were done in five different magnetic field directions, with $\phi = 315°$ (red), $\phi = 292.5°$ (orange), $\phi = 270°$ (green), $\phi = 241°$ (blue) and $\phi = 225°$ (purple).

To extract the corrections to the bulk g-factor, we then plotted these g-factors against $\phi$ and fitted a sinusoidal function with a period of 180°, yielding the mean value of the fit $|\bar{g}|$ and the anisotropic correction $\delta g_a$ as the amplitude of the fit. For this device, we obtain $|\bar{g}| \approx 0.396$ and $\delta g_a \approx 0.025$.

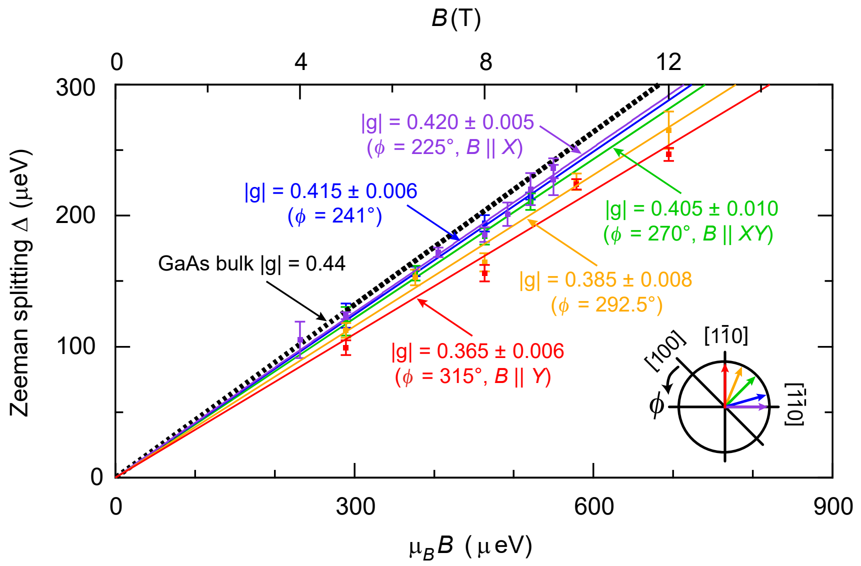


FIG. S4. Extracted Zeeman splittings $\Delta E_Z$ and absolute g-factors in device 2 for different in-plane magnetic field strengths and directions, given by the angle $\phi$. The corresponding crystallographic directions of the traces are marked in the inset, and the bulk g-factor of GaAs is indicated with a dashed line.

## Supplementary References

---

* These authors contributed equally.

† Present address: Laboratory for Physical Sciences, 8050 Greenmead Drive, College Park, MD 20740, USA.

‡ Present address: Physics Department, Colorado School of Mines, Golden, CO, 80401, USA.

[1] L. C. Camenzind, L. Yu, P. Stano, J. D. Zimmerman, A. C. Gossard, D. Loss, and D. M. Zumbühl, Phys. Rev. Lett. **122**, 207701 (2019).

[2] P. Stano, C.-H. Hsu, L. C. Camenzind, L. Yu, D. Zumbühl, and D. Loss, Phys. Rev. B **99**, 085308 (2019).

[3] P. Stano, C.-H. Hsu, M. Serina, L. C. Camenzind, D. M. Zumbühl, and D. Loss, Phys. Rev. B **98**, 195314 (2018).

[4] K. MacLean, S. Amasha, I. P. Radu, D. M. Zumbühl, M. A. Kastner, M. P. Hanson, and A. C. Gossard, Phys. Rev. Lett. **98**, 036802 (2007).

[5] S. Amasha, K. MacLean, I. P. Radu, D. M. Zumbühl, M. A. Kastner, M. P. Hanson, and A. C. Gossard, Phys. Rev. Lett. **100**, 046803 (2008).

[6] P. Stano and P. Jacquod, Phys. Rev. B **82**, 125309 (2010).

[7] C. B. Simmons, J. R. Prance, B. J. Van Bael, T. S. Koh, Z. Shi, D. E. Savage, M. G. Lagally, R. Joynt, M. Friesen, S. N. Coppersmith, and M. A. Eriksson, Phys. Rev. Lett. **106**, 156804 (2011).

[8] M. Yamagishi, N. Watase, M. Hashisaka, K. Muraki, and T. Fujisawa, Phys. Rev. B **90**, 035306 (2014).

[9] S. Amasha, K. MacLean, I. P. Radu, D. M. Zumbühl, M. A. Kastner, M. P. Hanson, and A. C. Gossard, Phys. Rev. B **78**, 041306 (2008).

[10] Y. V. Nazarov and Y. M. Blanter, Book (Cambridge University Press, Cambridge, 2009) p. 591.

[11] D. E. F. Biesinger, C. P. Scheller, B. Braunecker, J. Zimmerman, A. C. Gossard, and D. M. Zumbühl, Phys. Rev. Lett. **115**, 106804 (2015).
